# Supplementary material for: Robotic Vision for Human-Robot Interaction and Collaboration: A Survey and Systematic Review
Source: arXiv:2307.15363 source file (2023-07-28)
Supplement: Supplementary file 1 [file scratchpad_additional_includes.tex]

Rosenberger et al~\cite{rosenberger_object-independent_2020} safely grasp objects (e.g. banana, lemon, tin of tuna) from a human hand by first segmenting out human pixels from potential grasp locations using a Franka Panda arm.

Rosenberger et al~\cite{rosenberger_object-independent_2020} use a YOLOv3~\cite{} network for object detection, a fine tuned ResNet50~\cite{} network to segment a human hand from grasping locations on an object, and GG-CNN~\cite{} to to detect grasp locations of the segmented object. 

The EgoHands dataset~\cite{bambach_lending_2015} (15,000 images of hands) was used to train a hand detector~\cite{rosenberger_object-independent_2020}.

Pre-trained YOLOv3 to detect objects, RefineNet originally proposed by Lin [22], which was trained on the portion of the PASCAL dataset that belong to the class “Person” to detect person, hand segmentation network (per-pixel, hand or not, ResNet50 trained on custom dataset, GG-CNN to detect grasp pose, visual servoing for moving to object~\cite{rosenberger_object-independent_2020}

Kollmitz replaced by vasquez (was a duplicate paper)
Kollmitz et al\cite{kollmitz_deep_2019} classify the class label, 3D position and velocity of a person using a walking aid using a ResNet-50~\cite{he_deep_2016} and a hidden markov model (HMM). The region of interested was first extracted by the faster-RCNN, and the classifier network was pre-trained on ImageNet data and fine tuned with a custom dataset.

Hand waving has also been used to select a specific unmanned aerial vehicle from a team~\cite{monajjemi_hri_2013}. For instance, multiple unmanned aerial vehicles could detect a persons face direction, followed by robot selection when the person waves to a robot they are looking at directly. Deselection then occurs by waving with the opposite hand. The selected robots then respond to a command (e.g both hands waving down to land) ~\cite{monajjemi_hri_2013}.

Need to see if any other papers use these methods:
optic flow for hand wave detection~\cite{monajjemi_hri_2013},

 by creating a map using parallel tracking and mapping (PTAM)~\cite{monajjemi_hri_2013}
 
Almonfrey et al~\cite{almonfrey_flexible_2018} developed a vision network using four static cameras to create an intelligent work space, where a mobile robot can identify and avoid people.

Almonfrey et al~\cite{almonfrey_flexible_2018} use a vision network (4 static RGB cameras) to create an intelligent work space, where a Pioneer robot can localise itself, and follow or avoid people. 

Almonfrey et al~\cite{almonfrey_flexible_2018} train a person detectors using the INRIA dataset~\cite{dalal_histograms_2005}, containing over 1800 annotated human images.

Almonfrey et al~\cite{almonfrey_flexible_2018} compare their human detection method using a network of cameras to other methods to show they have a lower miss rate (fraction of total humans not identified), than other methods.

Gao et al~\cite{gao_user_2020} use a Gaussian mixture model to predict the motion of a human in an assisted dressing task~\cite{gao_user_2020}

From a study with 31 people in a robot assistive dressing experiment~\cite{gao_user_2020}, users were most comfortable with a method that combined a motion model, vision, and force feedback (compared to vision or force only modalities). Some users were happy to have a robot assisting them dressing.

For assistive dressing, combining a motion model, vision, and force feedback improved the reachability of a Baxter robot~\cite{gao_user_2020}. 

Mobile robot have been summoned by waving, and directed to a specific location by pointing~\cite{kahlouche_human_2019}.

Kahlouche et al~\cite{kahlouche_human_2019} fuse multiple classification methods (SVM, decision tree, and a MLP) using a voting process from an ensemble of classifiers.

TODO: replace with Vasquez:
Kollmitz et al found that RGB data performed better than DepthJet (colour-encoded depth image), and found that a VGG-CNN-M~\cite{chatfield_return_2014} provided a trade off between classification accuracy and processing speed (compared to ResNet-50~\cite{he_deep_2016} and GoogLeNet~\cite{szegedy_going_2015}) when classifying people with walking aids.
